# Supplementary material for: A Causal Mediation Model for Longitudinal Mediators and Survival Outcomes with an Application to Animal Behavior
Source: arXiv:2104.08344 source file (2022-02-12)
Supplement: Supplementary file 1 [file additionalreference.tex]

Anderson, M. and M. Marmot. 2012. The effects of promotions on heart disease: Evidence from Whitehall. The Economic Journal 122:555-589.

Case, A. and C. Paxson. 2011. The long reach of childhood health and circumstance: evidence from the Whitehall II Study. The Economic Journal 121:F183-F204.

Chandola, T., M. Bartley, A. Sacker, C. Jenkinson, and M. Marmot. 2003. Health selection in the Whitehall II study, UK. Social Science & Medicine 56:2059-2072.

Chartier, M. J., J. R. Walker, and B. Naimark. 2010. Separate and cumulative effects of adverse childhood experiences in predicting adult health and health care utilization. Child Abuse & Neglect 34:454-464.

Elovainio, M., J. E. Ferrie, A. Singh-Manoux, M. Shipley, G. D. Batty, J. Head, M. Hamer, M. Jokela, M. Virtanen, and E. Brunner. 2011. Socioeconomic differences in cardiometabolic factors: social causation or health-related selection? Evidence from the Whitehall II Cohort Study, 1991–2004. American journal of epidemiology 174:779-789.

Evans, G. W., D. Li, and S. S. Whipple. 2013. Cumulative risk and child development. Psychological bulletin 139:1342.

Felitti, V. J., R. F. Anda, D. Nordenberg, D. F. Williamson, A. M. Spitz, V. Edwards, M. P. Koss, and J. S. Marks. 1998. Relationship of childhood abuse and household dysfunction to many of the leading causes of death in adults: The adverse childhood experiences (ACE) study. American journal of preventive medicine 14:245-258.

Harper, S. and E. C. Strumpf. 2012. Commentary: Social EpidemiologyQuestionable Answers and Answerable Questions. Epidemiology (Cambridge, Mass.) 23:795-798.

Holt-Lunstad, J., T. B. Smith, M. Baker, T. Harris, and D. Stephenson. 2015. Loneliness and social isolation as risk factors for mortality: a meta-analytic review. Perspectives on psychological science 10:227-237.

Holt-Lunstad, J., T. B. Smith, and J. B. Layton. 2010. Social Relationships and Mortality Risk: A Meta-analytic Review. PLOS Medicine 7:e1000316.

Jia, H. and E. I. Lubetkin. 2020. Impact of adverse childhood experiences on quality-adjusted life expectancy in the US population. Child Abuse & Neglect 102:104418.

Kröger, H., E. Pakpahan, and R. Hoffmann. 2015. What causes health inequality? A systematic review on the relative importance of social causation and health selection. The European Journal of Public Health 25:951-960.

Næss, Ø., B. Claussen, and G. D. Smith. 2004. Relative impact of childhood and adulthood socioeconomic conditions on cause specific mortality in men. Journal of Epidemiology & Community Health 58:597-598.

Petruccelli, K., J. Davis, and T. Berman. 2019. Adverse childhood experiences and associated health outcomes: A systematic review and meta-analysis. Child Abuse & Neglect 97:104127.

Snyder-Mackler, N., J. R. Burger, L. Gaydosh, D. W. Belsky, G. A. Noppert, F. A. Campos, A. Bartolomucci, Y. C. Yang, A. E. Aiello, A. O’Rand, K. Mullan Harris, C. A. Shively, S. C. Alberts, and J. Tung. 2020. Social determinants of health and survival in humans and other animals. Science 368.

Warren, J. R. 2009. Socioeconomic status and health across the life course: a test of the social causation and health selection hypotheses. Social forces 87:2125-2153.
